# Supplementary material for: Assessment of the GLLB-SC potential for solid-state properties and attempts for improvement
Source: arXiv:1712.06508 ancillary file (2017-12-18)
Supplement: Supplementary file 1 [file Supplemental_Material.pdf]

# Supplemental Material for
# Assessment of the GLLB-SC potential for solid-state properties and attempts for improvement

Fabien Tran, Sohaib Ehsan, and Peter Blaha
*Institute of Materials Chemistry, Vienna University of Technology,*
*Getreidemarkt 9/165-TC, A-1060 Vienna, Austria*

[1] ICSD, Inorganic Crystal Structure Database, http://icsd.fiz-karlsruhe.de (accessed January, 2017).
[2] American Mineralogist Crystal Structure Database, http://rruff.geo.arizona.edu/AMS/amcsd.php (accessed January, 2017).
[3] P. Villars and J. Daams, J. Alloys Compd. **197**, 177 (1993).
[4] J. Heyd, J. E. Peralta, G. E. Scuseria, and R. L. Martin, J. Chem. Phys. **123**, 174101 (2005).
[5] J. M. Crowley, J. Tahir-Kheli, and W. A. Goddard, III, J. Phys. Chem. Lett. **7**, 1198 (2016).
[6] H. Haas and J. G. Correia, Hyperfine Interact. **198**, 133 (2010).
[7] M. J. Lucero, T. M. Henderson, and G. E. Scuseria, J. Phys.: Condens. Matter **24**, 145504 (2012).
[8] S. Bernstorff and V. Saile, Opt. Commun. **58**, 181 (1986).
[9] R. Gillen and J. Robertson, J. Phys.: Condens. Matter **25**, 165502 (2013).
[10] L. Schimka, J. Harl, and G. Kresse, J. Chem. Phys. **134**, 024116 (2011).
[11] D. Koller, P. Blaha, and F. Tran, J. Phys.: Condens. Matter **25**, 435503 (2013).
[12] J. H. Skone, M. Govoni, and G. Galli, Phys. Rev. B **89**, 195112 (2014).
[13] H. Shi, R. I. Eglitis, and G. Borstel, Phys. Rev. B **72**, 045109 (2005).
[14] J. Lee, A. Seko, K. Shitara, K. Nakayama, and I. Tanaka, Phys. Rev. B **93**, 115104 (2016).
[15] A. M. Ganose and D. O. Scanlon, J. Mater. Chem. C **4**, 1467 (2016).
[16] D. Groh, R. Pandey, M. B. Sahariah, E. Amzallag, I. Baraille, and M. Rérat, J. Phys. Chem. Solids **70**, 789 (2009).
[17] F. Tran and P. Blaha, J. Phys. Chem. A **121**, 3318 (2017).
[18] J. M. Zuo, P. Blaha, and K. Schwarz, J. Phys.: Condens. Matter **9**, 7541 (1997).

TABLE S1. Experimental[1–6] lattice constants (in Å) and angles (in degrees) of the unit cell for the solids considered in this work. When necessary, the positions of atoms (in internal units) are also indicated. The space group number is indicated in parenthesis. For $Cr_2O_3$, $Fe_2O_3$, MnO, FeO, CoO, NiO, and CuO the antiferromagnetic order leads to a lowering of the symmetry (second indicated space group). The first 76 solids (those before the horizontal line) constitute the test set for the band gap, while the other 11 solids are test cases for the magnetic moment or electric field gradient.

| Solid | $a$ | $b$ | $c$ | $\alpha$ | $\beta$ | $\gamma$ |
|---|---|---|---|---|---|---|
| Ne (225) | 4.470 | 4.470 | 4.470 | 90 | 90 | 90 |
| Ar (225) | 5.260 | 5.260 | 5.260 | 90 | 90 | 90 |
| Kr (225) | 5.640 | 5.640 | 5.640 | 90 | 90 | 90 |
| Xe (225) | 6.130 | 6.130 | 6.130 | 90 | 90 | 90 |
| C (227) | 3.567 | 3.567 | 3.567 | 90 | 90 | 90 |
| Si (227) | 5.430 | 5.430 | 5.430 | 90 | 90 | 90 |
| Ge (227) | 5.652 | 5.652 | 5.652 | 90 | 90 | 90 |
| $Al_2O_3$ (167) | 4.757 | 4.757 | 12.988 | 90 | 90 | 120 |
| Al(0,0,0.35218), O(0.30625,0,1/4) | | | | | | |
| SiC (216) | 4.358 | 4.358 | 4.358 | 90 | 90 | 90 |
| $SiO_2$ ($\alpha$-quartz,152) | 4.921 | 4.921 | 5.400 | 90 | 90 | 120 |
| Si(0.528,0,1/3), O(0.408,0.143,0.1193) | | | | | | |
| $SiO_2$ ($\beta$-cristobalite,227) | 7.126 | 7.126 | 7.126 | 90 | 90 | 90 |
| BN (216) | 3.616 | 3.616 | 3.616 | 90 | 90 | 90 |
| BP (216) | 4.538 | 4.538 | 4.538 | 90 | 90 | 90 |
| BAs (216) | 4.777 | 4.777 | 4.777 | 90 | 90 | 90 |
| AlN (216) | 4.342 | 4.342 | 4.342 | 90 | 90 | 90 |
| AlN (wurtzite,186) | 3.111 | 3.111 | 4.978 | 90 | 90 | 120 |
| Al(1/3,2/3,0), N(1/3,2/3,0.385) | | | | | | |
| AlP (216) | 5.463 | 5.463 | 5.463 | 90 | 90 | 90 |
| AlAs (216) | 5.661 | 5.661 | 5.661 | 90 | 90 | 90 |
| AlSb (216) | 6.136 | 6.136 | 6.136 | 90 | 90 | 90 |
| GaN (216) | 4.523 | 4.523 | 4.523 | 90 | 90 | 90 |
| GaN (wurtzite,186) | 3.180 | 3.180 | 5.166 | 90 | 90 | 120 |
| Ga(1/3,2/3,0), N(1/3,2/3,0.385) | | | | | | |
| GaP (216) | 5.451 | 5.451 | 5.451 | 90 | 90 | 90 |
| GaSb (216) | 6.096 | 6.096 | 6.096 | 90 | 90 | 90 |
| GaAs (216) | 5.648 | 5.648 | 5.648 | 90 | 90 | 90 |
| InN (wurtzite,186) | 3.533 | 3.533 | 5.693 | 90 | 90 | 120 |
| In(1/3,2/3,0), N(1/3,2/3,0.385) | | | | | | |
| InP (216) | 5.869 | 5.869 | 5.869 | 90 | 90 | 90 |
| InAs (216) | 6.058 | 6.058 | 6.058 | 90 | 90 | 90 |
| InSb (216) | 6.479 | 6.479 | 6.479 | 90 | 90 | 90 |
| $SnO_2$ (136) | 4.737 | 4.737 | 3.186 | 90 | 90 | 90 |
| Sn(0,0,0), O(0.30562,0.30562,0) | | | | | | |
| SnSe (62) | 11.500 | 4.154 | 4.446 | 90 | 90 | 90 |
| Sn(0.618,1/4,0.3957), Se(0.3559,1/4,0.0164) | | | | | | |
| SnTe (225) | 6.318 | 6.318 | 6.318 | 90 | 90 | 90 |
| $Sb_2Te_3$ (166) | 4.264 | 4.264 | 30.458 | 90 | 90 | 120 |
| Sb(0,0,0.3988), Te1(0,0,0.7872), Te2(0,0,0) | | | | | | |
| LiH (225) | 4.084 | 4.084 | 4.084 | 90 | 90 | 90 |
| LiF (225) | 4.010 | 4.010 | 4.010 | 90 | 90 | 90 |
| LiCl (225) | 5.106 | 5.106 | 5.106 | 90 | 90 | 90 |
| NaF (225) | 4.609 | 4.609 | 4.609 | 90 | 90 | 90 |
| NaCl (225) | 5.595 | 5.595 | 5.595 | 90 | 90 | 90 |
| KF (225) | 5.347 | 5.347 | 5.347 | 90 | 90 | 90 |
| KCl (225) | 6.293 | 6.293 | 6.293 | 90 | 90 | 90 |
| BeO (wurtzite,186) | 2.694 | 2.694 | 4.384 | 90 | 90 | 120 |
| Be(1/3,2/3,0), O(1/3,2/3,0.3778) | | | | | | |
| MgO (225) | 4.207 | 4.207 | 4.207 | 90 | 90 | 90 |
| MgS (216) | 5.622 | 5.622 | 5.622 | 90 | 90 | 90 |
| MgSe (225) | 5.400 | 5.400 | 5.400 | 90 | 90 | 90 |
| MgTe (216) | 6.420 | 6.420 | 6.420 | 90 | 90 | 90 |
| CaO (225) | 4.811 | 4.811 | 4.811 | 90 | 90 | 90 |
| $CaF_2$ (225) | 5.463 | 5.463 | 5.463 | 90 | 90 | 90 |
| BaS (225) | 6.389 | 6.389 | 6.389 | 90 | 90 | 90 |
| BaSe (225) | 6.595 | 6.595 | 6.595 | 90 | 90 | 90 |
| BaTe (225) | 7.007 | 7.007 | 7.007 | 90 | 90 | 90 |
| ScN (225) | 4.500 | 4.500 | 4.500 | 90 | 90 | 90 |
| $TiO_2$ (rutile,136) | 4.594 | 4.594 | 2.959 | 90 | 90 | 90 |
| Ti(0,0,0), O(0.305,0.305,0) | | | | | | |
| $TiO_2$ (anatase,141) | 3.785 | 3.785 | 9.512 | 90 | 90 | 90 |
| Ti(0,1/4,3/8), O(1/2,3/4,0.08314) | | | | | | |
| $SrTiO_3$ (221) | 3.901 | 3.901 | 3.901 | 90 | 90 | 90 |
| $VO_2$ ($M_1$,14) | 5.743 | 4.517 | 5.375 | 90 | 122.6 | 90 |
| V(0.242,0.975,0.025), O1(0.1,0.21,0.2), O2(0.39,0.69,0.29) | | | | | | |
| $Cr_2O_3$ (167,146) | 4.953 | 4.953 | 13.588 | 90 | 90 | 120 |
| Cr(0,0,0.3475), O(0.3058,0,1/4) | | | | | | |
| $Fe_2O_3$ (167,146) | 5.035 | 5.035 | 13.747 | 90 | 90 | 120 |
| Fe(0,0,0.35534), O(0.3056,0,1/4) | | | | | | |
| MnO (225,166) | 4.445 | 4.445 | 4.445 | 90 | 90 | 90 |
| FeO (225,166) | 4.334 | 4.334 | 4.334 | 90 | 90 | 90 |
| CoO (225,166) | 4.254 | 4.254 | 4.254 | 90 | 90 | 90 |
| NiO (225,166) | 4.171 | 4.171 | 4.171 | 90 | 90 | 90 |
| $Cu_2O$ (224) | 4.267 | 4.267 | 4.267 | 90 | 90 | 90 |
| CuSCN (160) | 3.856 | 3.856 | 16.452 | 90 | 90 | 120 |
| Cu(0,0,0), S(0.28904,0.28904,0.28904) | | | | | | |
| C(0.18674,0.18674,0.18674), N(0.1169,0.1169,0.1169) | | | | | | |
| CuCl (216) | 5.501 | 5.501 | 5.501 | 90 | 90 | 90 |
| CuBr (216) | 5.820 | 5.820 | 5.820 | 90 | 90 | 90 |
| CuI (216) | 6.063 | 6.063 | 6.063 | 90 | 90 | 90 |
| ZnO (wurtzite,186) | 3.258 | 3.258 | 5.220 | 90 | 90 | 120 |
| Zn(1/3,2/3,0), O(1/3,2/3,0.382) | | | | | | |
| ZnS (216) | 5.409 | 5.409 | 5.409 | 90 | 90 | 90 |
| ZnSe (216) | 5.668 | 5.668 | 5.668 | 90 | 90 | 90 |
| ZnTe (216) | 6.089 | 6.089 | 6.089 | 90 | 90 | 90 |
| $MoS_2$ (194) | 3.160 | 3.160 | 12.294 | 90 | 90 | 120 |
| Mo(1/3,2/3,1/4), S(1/3,2/3,0.621) | | | | | | |
| AgCl (225) | 5.546 | 5.546 | 5.546 | 90 | 90 | 90 |
| AgBr (225) | 5.772 | 5.772 | 5.772 | 90 | 90 | 90 |
| AgI (216) | 6.499 | 6.499 | 6.499 | 90 | 90 | 90 |
| CdS (216) | 5.818 | 5.818 | 5.818 | 90 | 90 | 90 |
| CdSe (216) | 6.052 | 6.052 | 6.052 | 90 | 90 | 90 |
| CdTe (216) | 6.480 | 6.480 | 6.480 | 90 | 90 | 90 |
| Ti (194) | 2.950 | 2.950 | 4.681 | 90 | 90 | 120 |
| Fe (229) | 2.867 | 2.867 | 2.867 | 90 | 90 | 90 |
| Co (194) | 2.507 | 2.507 | 4.070 | 90 | 90 | 120 |
| Ni (225) | 3.523 | 3.523 | 3.523 | 90 | 90 | 90 |
| Zn (194) | 2.655 | 2.655 | 4.853 | 90 | 90 | 120 |
| Zr (194) | 3.232 | 3.232 | 5.148 | 90 | 90 | 120 |
| Tc (194) | 2.741 | 2.741 | 4.398 | 90 | 90 | 120 |
| Ru (194) | 2.705 | 2.705 | 4.282 | 90 | 90 | 120 |
| Cd (194) | 2.963 | 2.963 | 5.519 | 90 | 90 | 120 |
| CuO (15,14) | 4.684 | 3.423 | 5.129 | 90 | 99.54 | 90 |
| Cu(1/4,1/4,0), O(0,0.4184,1/4) | | | | | | |
| $Cu_2Mg$ (227) | 7.061 | 7.061 | 7.061 | 90 | 90 | 90 |

TABLE S2. Calculated and experimental[5,7–16] band gaps (in eV). The contribution from the exchange derivative discontinuity to the GLLB-SC band gap is indicated in parenthesis. All results except the ones obtained with the BJLDA, LB94, and GLLB-SC methods are taken from Ref. 17.

| Solid | LDA | PBE | EV93PW91 | AK13 | Sloc | HLE16 | BJLDA | mBJLDA | LB94 | GLLB-SC | HSE06 | Expt. |
|---|---|---|---|---|---|---|---|---|---|---|---|---|
| Ne (225) | 11.42 | 11.58 | 11.21 | 19.98 | 18.30 | 15.06 | 13.88 | 22.33 | 14.12 | 22.13 (6.60) | 14.27 | 21.48 |
| Ar (225) | 8.18 | 8.70 | 9.26 | 15.13 | 12.57 | 11.74 | 9.65 | 13.84 | 9.32 | 14.98 (4.71) | 10.37 | 14.15 |
| Kr (225) | 6.76 | 7.26 | 7.95 | 12.82 | 10.61 | 10.09 | 7.98 | 10.80 | 7.78 | 12.39 (4.02) | 8.71 | 11.59 |
| Xe (225) | 5.78 | 6.24 | 7.03 | 10.67 | 9.02 | 8.80 | 6.77 | 8.48 | 6.64 | 10.25 (3.37) | 7.44 | 9.29 |
| C (227) | 4.10 | 4.14 | 4.31 | 4.78 | 5.18 | 4.55 | 4.41 | 4.92 | 4.15 | 5.46 (1.30) | 5.26 | 5.50 |
| Si (227) | 0.47 | 0.57 | 0.91 | 1.60 | 1.70 | 1.38 | 0.83 | 1.15 | 0.25 | 1.06 (0.34) | 1.17 | 1.17 |
| Ge (227) | 0.00 | 0.06 | 0.58 | 0.70 | 0.00 | 0.12 | 0.18 | 0.83 | 0.00 | 0.24 (0.06) | 0.82 | 0.74 |
| $Al_2O_3$ (167) | 6.19 | 6.26 | 6.67 | 7.92 | 7.30 | 7.20 | 7.04 | 8.34 | 6.88 | 9.82 (2.58) | 8.08 | 8.80 |
| SiC (216) | 1.32 | 1.36 | 1.52 | 2.18 | 2.83 | 2.06 | 1.81 | 2.25 | 1.67 | 2.56 (0.75) | 2.23 | 2.42 |
| $SiO_2$ ($\alpha$-quartz,152) | 5.70 | 5.93 | 6.47 | 8.17 | 7.58 | 7.53 | 6.82 | 8.70 | 6.72 | 9.88 (2.76) | 7.77 | 9.65 |
| $SiO_2$ ($\beta$-cristobalite,227) | 5.54 | 5.79 | 5.81 | 9.48 | 9.20 | 8.10 | 7.04 | 10.43 | 6.79 | 10.73 (2.96) | 7.39 | 8.90 |
| BN (216) | 4.35 | 4.47 | 4.82 | 5.67 | 6.18 | 5.38 | 4.95 | 5.80 | 4.86 | 6.66 (1.65) | 5.76 | 6.36 |
| BP (216) | 1.19 | 1.24 | 1.46 | 2.02 | 2.37 | 1.85 | 1.50 | 1.85 | 1.13 | 1.85 (0.53) | 1.98 | 2.10 |
| BAs (216) | 1.14 | 1.20 | 1.46 | 1.96 | 2.23 | 1.82 | 1.38 | 1.71 | 1.14 | 1.76 (0.50) | 1.86 | 1.46 |
| AlN (216) | 3.24 | 3.33 | 3.58 | 4.44 | 5.25 | 4.41 | 4.03 | 4.88 | 4.07 | 6.10 (1.82) | 4.55 | 4.90 |
| AlN (wurtzite,186) | 4.18 | 4.16 | 4.43 | 5.31 | 5.17 | 4.80 | 4.86 | 5.51 | 4.71 | 6.56 (1.89) | 5.49 | 6.19 |
| AlP (216) | 1.45 | 1.59 | 2.10 | 3.00 | 3.08 | 2.75 | 1.88 | 2.31 | 1.57 | 2.80 (0.92) | 2.30 | 2.50 |
| AlAs (216) | 1.35 | 1.45 | 1.90 | 2.76 | 1.95 | 2.55 | 1.75 | 2.13 | 1.14 | 2.55 (0.84) | 2.11 | 2.23 |
| AlSb (216) | 1.15 | 1.22 | 1.56 | 2.29 | 1.16 | 1.84 | 1.47 | 1.75 | 0.56 | 2.00 (0.67) | 1.80 | 1.69 |
| GaN (216) | 1.67 | 1.66 | 1.95 | 2.37 | 2.57 | 2.39 | 2.21 | 2.85 | 1.84 | 2.89 (0.84) | 2.85 | 3.28 |
| GaN (wurtzite,186) | 1.94 | 1.94 | 2.27 | 2.71 | 2.82 | 2.68 | 2.49 | 3.17 | 2.12 | 3.26 (0.93) | 3.15 | 3.50 |
| GaP (216) | 1.44 | 1.60 | 2.08 | 2.60 | 1.57 | 2.35 | 1.74 | 2.25 | 0.61 | 2.56 (0.78) | 2.28 | 2.35 |
| GaSb (216) | 0.00 | 0.11 | 0.60 | 0.76 | 0.00 | 0.26 | 0.23 | 0.95 | 0.00 | 0.32 (0.09) | 0.88 | 0.82 |
| GaAs (216) | 0.30 | 0.54 | 1.13 | 1.45 | 0.12 | 0.94 | 0.75 | 1.64 | 0.00 | 1.05 (0.29) | 1.40 | 1.52 |
| InN (wurtzite,186) | 0.02 | 0.03 | 0.18 | 0.56 | 0.73 | 0.60 | 0.28 | 0.89 | 0.04 | 0.37 (0.12) | 0.70 | 0.72 |
| InP (216) | 0.46 | 0.68 | 1.30 | 1.81 | 0.63 | 1.29 | 0.87 | 1.62 | 0.00 | 1.51 (0.45) | 1.43 | 1.42 |
| InAs (216) | 0.00 | 0.00 | 0.36 | 0.73 | 0.00 | 0.23 | 0.00 | 0.67 | 0.00 | 0.07 (0.02) | 0.45 | 0.42 |
| InSb (216) | 0.00 | 0.00 | 0.30 | 0.51 | 0.00 | 0.00 | 0.00 | 0.47 | 0.00 | 0.00 (0.00) | 0.45 | 0.24 |
| $SnO_2$ (136) | 1.09 | 1.24 | 1.64 | 2.20 | 1.40 | 1.62 | 1.85 | 3.19 | 1.09 | 3.33 (0.90) | 2.88 | 3.59 |
| SnSe (62) | 0.48 | 0.55 | 0.76 | 1.10 | 1.17 | 1.03 | 0.73 | 0.89 | 0.76 | 1.29 (0.39) | 0.98 | 0.90 |
| SnTe (225) | 0.09 | 0.07 | 0.07 | 0.22 | 0.74 | 0.47 | 0.10 | 0.15 | 0.41 | 0.04 (0.01) | 0.17 | 0.36 |
| $Sb_2Te_3$ (166) | 0.04 | 0.00 | 0.20 | 0.18 | 0.35 | 0.34 | 0.11 | 0.24 | 0.08 | 0.21 (0.06) | 0.31 | 0.28 |
| LiH (225) | 2.67 | 3.03 | 3.72 | 6.19 | 4.33 | 4.21 | 3.67 | 5.06 | 3.26 | 6.47 (2.12) | 4.06 | 4.94 |
| LiF (225) | 8.95 | 9.20 | 9.98 | 12.55 | 11.76 | 11.84 | 10.18 | 12.89 | 10.43 | 15.03 (4.07) | 11.46 | 14.20 |
| LiCl (225) | 6.06 | 6.41 | 7.42 | 9.78 | 8.08 | 8.56 | 6.98 | 8.64 | 6.70 | 10.47 (3.07) | 7.81 | 9.40 |
| NaF (225) | 6.05 | 6.41 | 7.17 | 11.10 | 9.36 | 9.44 | 7.49 | 11.46 | 7.42 | 12.45 (3.66) | 8.57 | 11.50 |
| NaCl (225) | 4.79 | 5.21 | 6.18 | 9.82 | 7.16 | 7.73 | 5.85 | 8.45 | 5.24 | 9.55 (2.98) | 6.61 | 8.50 |
| KF (225) | 5.79 | 6.17 | 6.82 | 10.98 | 9.19 | 8.91 | 7.18 | 10.40 | 7.18 | 12.42 (3.58) | 8.18 | 10.90 |
| KCl (225) | 4.75 | 5.19 | 6.02 | 9.79 | 7.38 | 7.59 | 5.84 | 8.48 | 5.30 | 9.89 (3.18) | 6.53 | 8.50 |
| BeO (wurtzite,186) | 7.58 | 7.65 | 8.22 | 9.42 | 9.38 | 8.91 | 8.51 | 9.66 | 8.67 | 11.36 (2.98) | 9.48 | 10.60 |
| MgO (225) | 4.69 | 4.78 | 5.17 | 6.69 | 6.11 | 5.91 | 5.60 | 7.13 | 5.50 | 8.31 (2.33) | 6.47 | 7.83 |
| MgS (216) | 3.29 | 3.57 | 4.50 | 6.21 | 4.76 | 5.26 | 4.08 | 5.17 | 3.43 | 6.46 (2.08) | 4.66 | 4.78 |
| MgSe (225) | 1.71 | 1.87 | 2.21 | 3.65 | 2.66 | 2.86 | 2.21 | 2.93 | 1.72 | 3.99 (1.20) | 2.74 | 2.47 |
| MgTe (216) | 2.27 | 2.51 | 3.22 | 4.74 | 3.19 | 3.68 | 2.88 | 3.61 | 2.12 | 4.70 (1.65) | 3.39 | 3.60 |
| CaO (225) | 3.49 | 3.67 | 4.07 | 5.03 | 4.36 | 4.63 | 4.06 | 5.35 | 3.50 | 7.33 (1.96) | 5.26 | 7.00 |
| $CaF_2$ (225) | 6.92 | 7.30 | 8.11 | 9.81 | 9.04 | 9.26 | 8.37 | 10.34 | 8.26 | 12.98 (3.63) | 9.37 | 11.80 |
| BaS (225) | 2.00 | 2.20 | 2.79 | 4.03 | 3.43 | 3.56 | 2.46 | 3.27 | 2.07 | 4.57 (1.53) | 3.11 | 3.88 |
| BaSe (225) | 1.82 | 1.97 | 2.50 | 3.68 | 3.17 | 3.25 | 2.23 | 2.86 | 1.96 | 4.08 (1.39) | 2.79 | 3.58 |
| BaTe (225) | 1.48 | 1.61 | 2.09 | 3.23 | 2.72 | 2.79 | 1.83 | 2.28 | 1.60 | 3.24 (1.14) | 2.31 | 3.08 |
| ScN (225) | 0.00 | 0.00 | 0.18 | 0.70 | 0.41 | 0.40 | 0.17 | 0.88 | 0.00 | 1.21 (0.33) | 0.90 | 0.90 |
| $TiO_2$ (rutile,136) | 1.80 | 1.89 | 2.03 | 2.23 | 1.44 | 1.75 | 1.97 | 2.56 | 1.56 | 3.77 (0.71) | 3.34 | 3.30 |
| $TiO_2$ (anatase,141) | 2.00 | 2.11 | 2.30 | 2.54 | 1.74 | 2.06 | 2.21 | 2.92 | 1.72 | 4.22 (0.87) | 3.57 | 3.40 |
| $SrTiO_3$ (221) | 1.78 | 1.88 | 2.06 | 2.34 | 1.61 | 1.87 | 2.02 | 2.68 | 1.55 | 3.86 (0.79) | 3.29 | 3.30 |
| $VO_2$ ($M_1$,14) | 0.00 | 0.00 | 0.00 | 0.00 | 0.00 | 0.00 | 0.00 | 0.51 | 0.00 | 0.23 (0.05) | 1.03 | 0.60 |
| $Cr_2O_3$ (167,146) | 1.20 | 1.63 | 1.88 | 2.35 | 1.46 | 1.53 | 1.85 | 3.68 | 0.76 | 3.07 (0.88) | 4.42 | 3.40 |
| $Fe_2O_3$ (167,146) | 0.33 | 0.56 | 0.88 | 1.50 | 1.49 | 1.70 | 0.68 | 2.35 | 0.00 | 4.81 (0.76) | 3.24 | 2.20 |
| MnO (225,166) | 0.74 | 0.86 | 1.23 | 2.56 | 3.71 | 3.26 | 1.39 | 2.94 | 0.15 | 3.79 (1.18) | 2.85 | 3.90 |
| FeO (225,166) | 0.00 | 0.00 | 0.10 | 0.84 | 0.20 | 0.13 | 0.29 | 1.84 | 0.00 | 0.00 (0.00) | 2.35 | 2.40 |
| CoO (225,166) | 0.00 | 0.00 | 0.24 | 1.35 | 0.43 | 0.34 | 0.62 | 3.13 | 0.00 | 1.85 (0.56) | 3.48 | 2.50 |
| NiO (225,166) | 0.43 | 0.95 | 1.35 | 2.08 | 1.21 | 1.23 | 1.59 | 4.14 | 0.00 | 3.07 (0.77) | 4.37 | 4.30 |
| $Cu_2O$ (224) | 0.53 | 0.53 | 0.57 | 0.84 | 1.27 | 0.81 | 0.77 | 0.81 | 1.13 | 1.10 (0.32) | 1.98 | 2.17 |
| CuSCN (160) | 2.01 | 2.23 | 2.46 | 2.78 | 3.64 | 3.24 | 2.57 | 2.79 | 2.68 | 4.08 (1.10) | 3.60 | 3.94 |
| CuCl (216) | 0.33 | 0.47 | 0.98 | 1.95 | 3.78 | 2.95 | 1.16 | 1.69 | 1.82 | 2.52 (0.86) | 2.37 | 3.40 |
| CuBr (216) | 0.20 | 0.36 | 0.89 | 1.76 | 3.38 | 2.69 | 1.00 | 1.56 | 1.46 | 2.12 (0.73) | 2.15 | 3.07 |
| CuI (216) | 0.95 | 1.12 | 1.66 | 2.36 | 3.32 | 2.98 | 1.67 | 2.20 | 1.71 | 2.62 (0.82) | 2.65 | 3.12 |
| ZnO (wurtzite,186) | 0.74 | 0.81 | 1.27 | 2.06 | 3.21 | 2.81 | 1.65 | 2.65 | 1.81 | 2.57 (0.81) | 2.50 | 3.44 |
| ZnS (216) | 1.84 | 2.09 | 2.81 | 3.67 | 3.13 | 3.54 | 2.57 | 3.65 | 1.71 | 3.70 (1.08) | 3.30 | 3.84 |
| ZnSe (216) | 1.02 | 1.27 | 1.97 | 2.67 | 2.04 | 2.50 | 1.70 | 2.75 | 0.69 | 2.37 (0.70) | 2.37 | 2.82 |
| ZnTe (216) | 1.04 | 1.27 | 1.84 | 2.33 | 1.54 | 2.08 | 1.59 | 2.42 | 0.43 | 2.07 (0.59) | 2.25 | 2.39 |
| $MoS_2$ (194) | 0.79 | 0.86 | 1.02 | 1.25 | 1.18 | 1.21 | 0.91 | 1.08 | 0.83 | 1.39 (0.38) | 1.41 | 1.29 |
| AgCl (225) | 0.62 | 0.92 | 1.74 | 2.82 | 3.39 | 3.31 | 1.57 | 2.95 | 1.36 | 2.45 (0.80) | 2.41 | 3.25 |
| AgBr (225) | 0.38 | 0.67 | 1.48 | 2.44 | 2.76 | 2.77 | 1.26 | 2.50 | 0.92 | 1.87 (0.61) | 2.01 | 2.71 |
| AgI (216) | 1.05 | 1.34 | 2.02 | 3.02 | 3.15 | 3.14 | 1.76 | 2.77 | 1.33 | 2.54 (0.81) | 2.48 | 2.91 |
| CdS (216) | 0.88 | 1.16 | 1.91 | 2.84 | 2.21 | 2.60 | 1.51 | 2.67 | 0.69 | 2.41 (0.75) | 2.14 | 2.50 |
| CdSe (216) | 0.36 | 0.63 | 1.36 | 2.14 | 1.46 | 1.87 | 0.92 | 1.99 | 0.02 | 1.52 (0.47) | 1.52 | 1.85 |
| CdTe (216) | 0.51 | 0.76 | 1.39 | 1.98 | 1.12 | 1.61 | 0.96 | 1.79 | 0.00 | 1.46 (0.44) | 1.57 | 1.61 |

TABLE S3. Calculated and experimental form factors (in e/atom) of Si. See Ref. 18 for details.

| *hkl* | LDA | PBE | EV93PW91 | AK13 | Sloc | HLE16 | BJLDA | mBJLDA | LB94 | GLLB-SC | HSE06 | Expt. |
|---|---|---|---|---|---|---|---|---|---|---|---|---|
| 111 | 10.5987 | 10.6011 | 10.6158 | 10.6616 | 10.8237 | 10.7151 | 10.6171 | 10.6341 | 10.6459 | 10.5957 | 10.6061 | 10.6025(29) |
| 220 | 8.3939 | 8.3881 | 8.3664 | 8.3521 | 8.5209 | 8.4416 | 8.3857 | 8.3749 | 8.4655 | 8.3892 | 8.3868 | 8.3881(22) |
| 311 | 7.6902 | 7.6877 | 7.6747 | 7.6510 | 7.7656 | 7.7326 | 7.6746 | 7.6549 | 7.7724 | 7.6951 | 7.6840 | 7.6814(19) |
| 222 | 0.1604 | 0.1641 | 0.1651 | 0.1927 | 0.2076 | 0.1813 | 0.1937 | 0.2204 | 0.1178 | 0.1805 | 0.1756 | 0.182(1) |
| 400 | 6.9935 | 7.0009 | 7.0078 | 7.0070 | 7.0741 | 7.0683 | 7.0011 | 6.9996 | 7.0466 | 7.0321 | 7.0040 | 6.9958(12) |
| 331 | 6.7012 | 6.7112 | 6.7157 | 6.7375 | 6.8191 | 6.7919 | 6.7303 | 6.7483 | 6.7239 | 6.7581 | 6.7201 | 6.7264(20) |
| 422 | 6.0887 | 6.1011 | 6.1130 | 6.1296 | 6.1971 | 6.1886 | 6.1081 | 6.1212 | 6.1180 | 6.1495 | 6.1060 | 6.1123(22) |
| 333 | 5.7550 | 5.7688 | 5.7847 | 5.7982 | 5.8560 | 5.8587 | 5.7695 | 5.7807 | 5.7873 | 5.8176 | 5.7705 | 5.7806(21) |
| 511 | 5.7764 | 5.7894 | 5.8028 | 5.8189 | 5.8873 | 5.8813 | 5.7926 | 5.8046 | 5.8063 | 5.8383 | 5.7937 | 5.7906(27) |
| 440 | 5.3121 | 5.3247 | 5.3351 | 5.3524 | 5.4318 | 5.4183 | 5.3273 | 5.3408 | 5.3377 | 5.3761 | 5.3290 | 5.3324(20) |
| 531 | 5.0472 | 5.0596 | 5.0703 | 5.0866 | 5.1649 | 5.1535 | 5.0595 | 5.0717 | 5.0736 | 5.1104 | 5.0627 | 5.0655(17) |
| 620 | 4.6553 | 4.6666 | 4.6751 | 4.6896 | 4.7752 | 4.7599 | 4.6639 | 4.6742 | 4.6823 | 4.7152 | 4.6691 | 4.6707(9) |
| 533 | 4.4441 | 4.4542 | 4.4607 | 4.4730 | 4.5672 | 4.5461 | 4.4509 | 4.4595 | 4.4723 | 4.5005 | 4.4570 | 4.4552(11) |
| 444 | 4.1078 | 4.1172 | 4.1225 | 4.1340 | 4.2264 | 4.2057 | 4.1123 | 4.1203 | 4.1346 | 4.1620 | 4.1189 | 4.1239(18) |
| 711 | 3.9210 | 3.9299 | 3.9344 | 3.9451 | 4.0363 | 4.0159 | 3.9241 | 3.9314 | 3.9476 | 3.9737 | 3.9313 | 3.9282(22) |
| 551 | 3.9241 | 3.9328 | 3.9366 | 3.9467 | 4.0416 | 4.0188 | 3.9275 | 3.9347 | 3.9513 | 3.9763 | 3.9346 | 3.9349(34) |
| 642 | 3.6419 | 3.6496 | 3.6521 | 3.6612 | 3.7547 | 3.7314 | 3.6434 | 3.6496 | 3.6681 | 3.6908 | 3.6509 | 3.6558(54) |
| 731 | 3.4866 | 3.4938 | 3.4952 | 3.5034 | 3.5973 | 3.5729 | 3.4873 | 3.4929 | 3.5127 | 3.5334 | 3.4950 | 3.4919(11) |
| 553 | 3.4877 | 3.4951 | 3.4969 | 3.5060 | 3.5974 | 3.5740 | 3.4884 | 3.4945 | 3.5121 | 3.5351 | 3.4961 | 3.5055(14) |
| 800 | 3.2454 | 3.2518 | 3.2524 | 3.2593 | 3.3501 | 3.3261 | 3.2446 | 3.2491 | 3.2708 | 3.2889 | 3.2526 | 3.2485(34) |
| 733 | 3.1142 | 3.1201 | 3.1201 | 3.1265 | 3.2156 | 3.1916 | 3.1126 | 3.1167 | 3.1385 | 3.1557 | 3.1208 | 3.1270(14) |
| 822 | 2.9096 | 2.9146 | 2.9135 | 2.9187 | 3.0063 | 2.9816 | 2.9072 | 2.9103 | 2.9337 | 2.9476 | 2.9153 | 2.9111(15) |
| 660 | 2.9097 | 2.9147 | 2.9136 | 2.9188 | 3.0065 | 2.9817 | 2.9073 | 2.9105 | 2.9339 | 2.9476 | 2.9154 | 2.9143(16) |
| 555 | 2.7932 | 2.7978 | 2.7962 | 2.8004 | 2.8869 | 2.8622 | 2.7903 | 2.7927 | 2.8183 | 2.8290 | 2.7983 | 2.8009(21) |
| 751 | 2.7968 | 2.8014 | 2.7999 | 2.8046 | 2.8904 | 2.8657 | 2.7939 | 2.7967 | 2.8203 | 2.8329 | 2.8021 | 2.8006(25) |
| 840 | 2.6211 | 2.6251 | 2.6229 | 2.6268 | 2.7094 | 2.6850 | 2.6176 | 2.6197 | 2.6440 | 2.6542 | 2.6256 | 2.6200(7) |
| 911 | 2.5232 | 2.5269 | 2.5244 | 2.5278 | 2.6081 | 2.5841 | 2.5193 | 2.5209 | 2.5455 | 2.5546 | 2.5273 | 2.5325(8) |
| 753 | 2.5217 | 2.5254 | 2.5229 | 2.5262 | 2.6068 | 2.5828 | 2.5178 | 2.5194 | 2.5447 | 2.5530 | 2.5258 | 2.5274(29) |
| 664 | 2.3724 | 2.3755 | 2.3725 | 2.3753 | 2.4523 | 2.4287 | 2.3681 | 2.3692 | 2.3940 | 2.4010 | 2.3760 | 2.3677(9) |
| 844 | 2.1574 | 2.1598 | 2.1563 | 2.1584 | 2.2292 | 2.2069 | 2.1525 | 2.1529 | 2.1775 | 2.1820 | 2.1601 | 2.1506(24) |
| 880 | 1.5365 | 1.5372 | 1.5330 | 1.5338 | 1.5820 | 1.5655 | 1.5310 | 1.5296 | 1.5517 | 1.5492 | 1.5372 | 1.5325(26) |

TABLE S4. Calculated and experimental[5,7–16] band gaps (in eV). The contribution from the exchange derivative discontinuity is indicated in parenthesis.

| | GLLB | | | | | | | |
|---|---|---|---|---|---|---|---|---|
| | SC | LDA-x-hole | SCAN-x-hole | BR89-x-hole | PBEsol-x-resp | SCAN-x-resp | SCAN-x-hole+resp | Expt. |
| Ne (225) | 22.13 (6.60) | 21.90 (6.57) | 24.57 (7.14) | 21.69 (6.49) | 25.32 (9.53) | 21.29 (6.02) | 23.59 (6.45) | 21.48 |
| Ar (225) | 14.98 (4.71) | 15.21 (4.78) | 17.68 (5.38) | 13.76 (4.38) | 16.57 (6.06) | 14.32 (4.35) | 16.90 (4.95) | 14.15 |
| Kr (225) | 12.39 (4.02) | 12.59 (4.08) | 14.68 (4.61) | 11.35 (3.74) | 13.61 (5.03) | 11.79 (3.71) | 13.99 (4.25) | 11.59 |
| Xe (225) | 10.25 (3.37) | 10.37 (3.41) | 12.10 (3.86) | 9.34 (3.12) | 11.11 (4.07) | 9.69 (3.09) | 11.47 (3.55) | 9.29 |
| C (227) | 5.46 (1.30) | 5.43 (1.29) | 6.11 (1.44) | 5.15 (1.23) | 5.44 (1.33) | 5.28 (1.26) | 5.89 (1.40) | 5.50 |
| Si (227) | 1.06 (0.34) | 1.22 (0.39) | 2.19 (0.70) | 0.38 (0.12) | 1.17 (0.39) | 0.81 (0.26) | 1.88 (0.60) | 1.17 |
| Ge (227) | 0.24 (0.06) | 0.79 (0.23) | 1.31 (0.38) | 0.00 (0.00) | 0.55 (0.15) | 0.07 (0.02) | 1.10 (0.32) | 0.74 |
| $Al_2O_3$ (167) | 9.82 (2.58) | 9.57 (2.53) | 10.86 (2.84) | 9.76 (2.55) | 10.02 (2.74) | 9.41 (2.42) | 10.37 (2.65) | 8.80 |
| SiC (216) | 2.56 (0.75) | 2.44 (0.72) | 3.51 (1.02) | 2.24 (0.66) | 2.53 (0.77) | 2.25 (0.66) | 3.15 (0.91) | 2.42 |
| $SiO_2$ ($\alpha$-quartz,152) | 9.88 (2.76) | 9.71 (2.71) | 11.23 (3.06) | 9.83 (2.77) | 10.42 (3.17) | 9.45 (2.59) | 10.73 (2.87) | 9.65 |
| $SiO_2$ ($\beta$-cristobalite,227) | 10.73 (2.96) | 10.97 (3.00) | 12.65 (3.37) | 10.38 (2.90) | 12.45 (4.04) | 10.05 (2.67) | 11.91 (3.05) | 8.90 |
| BN (216) | 6.66 (1.65) | 6.52 (1.62) | 7.77 (1.91) | 6.23 (1.55) | 6.68 (1.71) | 6.29 (1.54) | 7.35 (1.79) | 6.36 |
| BP (216) | 1.85 (0.53) | 1.89 (0.54) | 2.70 (0.76) | 1.40 (0.40) | 1.86 (0.55) | 1.64 (0.47) | 2.43 (0.69) | 2.10 |
| BAs (216) | 1.76 (0.50) | 1.82 (0.51) | 2.37 (0.67) | 1.38 (0.39) | 1.80 (0.52) | 1.58 (0.45) | 2.16 (0.60) | 1.46 |
| AlN (216) | 6.10 (1.82) | 5.83 (1.75) | 7.32 (2.15) | 5.85 (1.74) | 6.15 (1.89) | 5.65 (1.63) | 6.81 (1.95) | 4.90 |
| AlN (wurtzite,186) | 6.56 (1.89) | 6.33 (1.83) | 7.38 (2.11) | 6.61 (1.89) | 6.61 (1.96) | 6.22 (1.76) | 6.97 (1.96) | 6.19 |
| AlP (216) | 2.80 (0.92) | 2.85 (0.94) | 3.99 (1.30) | 2.09 (0.70) | 2.91 (0.99) | 2.47 (0.81) | 3.62 (1.17) | 2.50 |
| AlAs (216) | 2.55 (0.84) | 2.57 (0.85) | 3.48 (1.13) | 2.11 (0.70) | 2.66 (0.91) | 2.26 (0.73) | 3.14 (1.01) | 2.23 |
| AlSb (216) | 2.00 (0.67) | 2.05 (0.68) | 2.76 (0.90) | 1.68 (0.56) | 2.11 (0.73) | 1.75 (0.58) | 2.49 (0.81) | 1.69 |
| GaN (216) | 2.89 (0.84) | 2.82 (0.82) | 3.60 (1.04) | 2.96 (0.86) | 2.94 (0.89) | 2.67 (0.77) | 3.29 (0.94) | 3.28 |
| GaN (wurtzite,186) | 3.26 (0.93) | 3.19 (0.92) | 3.97 (1.13) | 3.31 (0.95) | 3.32 (0.99) | 3.03 (0.86) | 3.66 (1.03) | 3.50 |
| GaP (216) | 2.56 (0.78) | 2.72 (0.82) | 3.56 (1.07) | 1.85 (0.57) | 2.72 (0.86) | 2.31 (0.70) | 3.26 (0.98) | 2.35 |
| GaSb (216) | 0.32 (0.09) | 0.88 (0.24) | 1.55 (0.46) | 0.00 (0.00) | 0.59 (0.17) | 0.14 (0.04) | 1.33 (0.39) | 0.82 |
| GaAs (216) | 1.05 (0.29) | 1.56 (0.42) | 2.42 (0.65) | 0.13 (0.04) | 1.33 (0.38) | 0.81 (0.22) | 2.08 (0.56) | 1.52 |
| InN (wurtzite,186) | 0.37 (0.12) | 0.35 (0.11) | 1.14 (0.37) | 0.32 (0.11) | 0.42 (0.14) | 0.17 (0.06) | 0.84 (0.27) | 0.72 |
| InP (216) | 1.51 (0.45) | 1.89 (0.56) | 2.82 (0.82) | 0.64 (0.19) | 1.78 (0.55) | 1.24 (0.37) | 2.45 (0.71) | 1.42 |
| InAs (216) | 0.07 (0.02) | 0.55 (0.16) | 1.37 (0.40) | 0.00 (0.00) | 0.35 (0.11) | 0.00 (0.00) | 1.05 (0.30) | 0.42 |
| InSb (216) | 0.00 (0.00) | 0.53 (0.15) | 1.15 (0.32) | 0.00 (0.00) | 0.27 (0.08) | 0.00 (0.00) | 0.90 (0.25) | 0.24 |
| $SnO_2$ (136) | 3.33 (0.90) | 3.27 (0.89) | 4.62 (1.23) | 3.12 (0.85) | 3.53 (1.00) | 3.04 (0.83) | 4.24 (1.13) | 3.59 |
| SnSe (62) | 1.29 (0.39) | 1.06 (0.33) | 1.45 (0.44) | 1.13 (0.35) | 1.25 (0.40) | 1.13 (0.34) | 1.30 (0.40) | 0.90 |
| SnTe (225) | 0.04 (0.01) | 0.19 (0.06) | 0.17 (0.05) | 0.08 (0.03) | 0.04 (0.01) | 0.12 (0.04) | 0.00 (0.00) | 0.36 |
| $Sb_2Te_3$ (166) | 0.21 (0.06) | 0.18 (0.05) | 0.40 (0.12) | 0.06 (0.02) | 0.23 (0.07) | 0.09 (0.03) | 0.38 (0.11) | 0.28 |
| LiH (225) | 6.47 (2.12) | 6.35 (2.09) | 9.22 (2.95) | 4.85 (1.61) | 6.90 (2.35) | 5.85 (1.89) | 8.60 (2.72) | 4.94 |
| LiF (225) | 15.03 (4.07) | 14.60 (3.99) | 16.38 (4.39) | 14.87 (4.01) | 15.61 (4.57) | 14.52 (3.81) | 15.79 (4.11) | 14.20 |
| LiCl (225) | 10.47 (3.07) | 10.38 (3.06) | 12.24 (3.53) | 9.53 (2.82) | 10.91 (3.39) | 9.90 (2.82) | 11.60 (3.25) | 9.40 |
| NaF (225) | 12.45 (3.66) | 12.20 (3.62) | 14.30 (4.12) | 12.05 (3.54) | 13.52 (4.42) | 11.85 (3.37) | 13.61 (3.79) | 11.50 |
| NaCl (225) | 9.55 (2.98) | 9.63 (3.02) | 11.72 (3.57) | 8.38 (2.65) | 10.32 (3.49) | 8.93 (2.71) | 11.02 (3.26) | 8.50 |
| KF (225) | 12.42 (3.58) | 12.29 (3.56) | 14.32 (4.01) | 12.06 (3.47) | 13.85 (4.55) | 11.82 (3.30) | 13.61 (3.68) | 10.90 |
| KCl (225) | 9.89 (3.18) | 10.09 (3.25) | 12.16 (3.78) | 8.78 (2.86) | 10.98 (3.94) | 9.32 (2.91) | 11.48 (3.46) | 8.50 |
| BeO (wurtzite,186) | 11.36 (2.98) | 10.97 (2.89) | 12.34 (3.23) | 11.43 (2.98) | 11.45 (3.13) | 10.92 (2.79) | 11.84 (3.02) | 10.60 |
| MgO (225) | 8.31 (2.33) | 8.02 (2.27) | 9.45 (2.63) | 8.16 (2.28) | 8.54 (2.49) | 7.84 (2.14) | 8.92 (2.41) | 7.83 |
| MgS (216) | 6.46 (2.08) | 6.50 (2.10) | 8.12 (2.67) | 5.55 (1.80) | 6.98 (2.46) | 5.96 (1.87) | 7.68 (2.49) | 4.78 |
| MgSe (225) | 3.99 (1.20) | 4.14 (1.24) | 5.14 (1.53) | 3.24 (0.99) | 4.36 (1.35) | 3.57 (1.06) | 4.69 (1.38) | 2.47 |
| MgTe (216) | 4.70 (1.65) | 4.69 (1.64) | 5.63 (1.94) | 3.77 (1.24) | 4.92 (1.81) | 4.15 (1.30) | 5.26 (1.79) | 3.60 |
| CaO (225) | 7.33 (1.96) | 7.46 (2.02) | 8.47 (2.20) | 6.80 (1.83) | 7.86 (2.25) | 7.07 (1.86) | 8.21 (2.10) | 7.00 |
| $CaF_2$ (225) | 12.98 (3.63) | 12.74 (3.59) | 14.78 (4.06) | 12.79 (3.57) | 13.99 (4.40) | 12.38 (3.35) | 14.09 (3.74) | 11.80 |
| BaS (225) | 4.57 (1.53) | 4.76 (1.60) | 5.86 (1.90) | 3.81 (1.30) | 4.98 (1.77) | 4.29 (1.42) | 5.55 (1.78) | 3.88 |
| BaSe (225) | 4.08 (1.39) | 4.22 (1.44) | 5.13 (1.70) | 3.52 (1.21) | 4.43 (1.60) | 3.81 (1.28) | 4.83 (1.58) | 3.58 |
| BaTe (225) | 3.24 (1.14) | 3.35 (1.18) | 4.12 (1.42) | 2.77 (0.98) | 3.52 (1.30) | 2.98 (1.03) | 3.83 (1.31) | 3.08 |
| ScN (225) | 1.21 (0.33) | 1.37 (0.37) | 2.16 (0.57) | 0.64 (0.18) | 1.41 (0.40) | 1.01 (0.27) | 1.94 (0.50) | 0.90 |
| $TiO_2$ (rutile,136) | 3.77 (0.71) | 3.96 (0.76) | 4.29 (0.80) | 3.46 (0.67) | 4.05 (0.81) | 3.76 (0.72) | 4.27 (0.81) | 3.30 |
| $TiO_2$ (anatase,141) | 4.22 (0.87) | 4.42 (0.91) | 4.82 (0.96) | 3.85 (0.81) | 4.53 (0.99) | 4.19 (0.87) | 4.79 (0.97) | 3.40 |
| $SrTiO_3$ (221) | 3.86 (0.79) | 4.08 (0.88) | 4.51 (0.94) | 3.57 (0.80) | 4.20 (0.96) | 3.82 (0.79) | 4.44 (0.91) | 3.30 |
| $VO_2$ ($M_1$,14) | 0.23 (0.05) | 0.33 (0.08) | 0.94 (0.24) | 0.00 (0.00) | 0.35 (0.09) | 0.03 (0.01) | 0.84 (0.19) | 0.60 |
| $Cr_2O_3$ (167,146) | 3.07 (0.88) | 3.15 (0.90) | 4.29 (1.19) | 2.73 (0.79) | 3.18 (0.94) | 2.84 (0.84) | 4.04 (1.15) | 3.40 |
| $Fe_2O_3$ (167,146) | 4.81 (0.76) | 5.59 (0.90) | 5.99 (0.89) | 3.77 (0.61) | 5.52 (0.92) | 4.85 (0.78) | 6.03 (0.92) | 2.20 |
| MnO (225,166) | 3.79 (1.18) | 3.33 (1.04) | 4.90 (1.51) | 3.95 (1.21) | 3.82 (1.24) | 3.34 (1.02) | 4.37 (1.32) | 3.90 |
| FeO (225,166) | 0.00 (0.00) | 0.00 (0.00) | 0.95 (0.27) | 0.19 (0.06) | 0.00 (0.00) | 0.00 (0.00) | 0.10 (0.03) | 2.40 |
| CoO (225,166) | 1.85 (0.56) | 0.85 (0.26) | 3.19 (0.93) | 1.09 (0.34) | 1.57 (0.49) | 1.17 (0.35) | 2.45 (0.70) | 2.50 |
| NiO (225,166) | 3.07 (0.77) | 3.53 (1.09) | 5.50 (1.66) | 2.33 (0.62) | 3.31 (0.86) | 2.61 (0.68) | 4.93 (1.46) | 4.30 |
| $Cu_2O$ (224) | 1.10 (0.32) | 0.84 (0.25) | 1.22 (0.36) | 1.33 (0.39) | 1.04 (0.32) | 0.99 (0.29) | 1.09 (0.32) | 2.17 |
| CuSCN (160) | 4.08 (1.10) | 4.08 (1.10) | 4.57 (1.21) | 3.95 (1.07) | 4.31 (1.24) | 3.96 (1.12) | 4.45 (1.20) | 3.94 |
| CuCl (216) | 2.52 (0.86) | 2.12 (0.73) | 3.55 (1.19) | 2.66 (0.89) | 2.64 (0.96) | 2.11 (0.70) | 3.06 (1.00) | 3.40 |
| CuBr (216) | 2.12 (0.73) | 1.83 (0.64) | 3.24 (1.08) | 2.13 (0.72) | 2.25 (0.82) | 1.73 (0.58) | 2.76 (0.91) | 3.07 |
| CuI (216) | 2.62 (0.82) | 2.50 (0.79) | 3.66 (1.13) | 2.42 (0.76) | 2.75 (0.91) | 2.28 (0.70) | 3.25 (0.98) | 3.12 |
| ZnO (wurtzite,186) | 2.57 (0.81) | 2.23 (0.71) | 3.57 (1.12) | 2.80 (0.88) | 2.62 (0.88) | 2.22 (0.69) | 3.14 (0.96) | 3.44 |
| ZnS (216) | 3.70 (1.08) | 3.84 (1.13) | 5.18 (1.50) | 3.02 (0.89) | 3.93 (1.21) | 3.32 (0.96) | 4.71 (1.34) | 3.84 |
| ZnSe (216) | 2.37 (0.70) | 2.62 (0.78) | 3.83 (1.11) | 1.66 (0.50) | 2.62 (0.81) | 2.03 (0.59) | 3.39 (0.97) | 2.82 |
| ZnTe (216) | 2.07 (0.59) | 2.40 (0.68) | 3.34 (0.93) | 1.37 (0.40) | 2.31 (0.69) | 1.80 (0.51) | 2.98 (0.82) | 2.39 |
| $MoS_2$ (194) | 1.39 (0.38) | 1.43 (0.39) | 1.70 (0.46) | 1.19 (0.33) | 1.45 (0.41) | 1.31 (0.36) | 1.62 (0.45) | 1.29 |
| AgCl (225) | 2.45 (0.80) | 2.35 (0.77) | 4.14 (1.32) | 1.89 (0.62) | 2.59 (0.89) | 1.97 (0.64) | 3.57 (1.11) | 3.25 |
| AgBr (225) | 1.87 (0.61) | 1.85 (0.60) | 3.48 (1.10) | 1.26 (0.42) | 2.01 (0.69) | 1.43 (0.46) | 2.95 (0.91) | 2.71 |
| AgI (216) | 2.54 (0.81) | 2.70 (0.86) | 3.94 (1.22) | 1.96 (0.63) | 2.82 (0.96) | 2.18 (0.69) | 3.48 (1.06) | 2.91 |
| CdS (216) | 2.41 (0.75) | 2.66 (0.82) | 4.00 (1.21) | 1.60 (0.50) | 2.71 (0.89) | 2.05 (0.63) | 3.52 (1.05) | 2.50 |
| CdSe (216) | 1.52 (0.47) | 1.83 (0.57) | 3.02 (0.91) | 0.69 (0.22) | 1.81 (0.59) | 1.19 (0.36) | 2.58 (0.77) | 1.85 |
| CdTe (216) | 1.46 (0.44) | 1.83 (0.55) | 2.76 (0.81) | 0.64 (0.20) | 1.74 (0.55) | 1.20 (0.36) | 2.40 (0.69) | 1.61 |
